# Supplementary material for: Learning to Sparsify Travelling Salesman Problem Instances
Source: arXiv:2104.09345 source file (2021-04-19)
Supplement: Supplementary file 1 [file appendices.tex]

\begin{subappendices}
\section{MWST Extraction}
\label{sec:mwstextraction}

The extraction of the minimum-weight spanning trees in succession necessitates the removal from consideration those that have been already identified in a minimum spanning tree. Each time these edges are removed, a unique minimum spanning tree can be determined in the resultant pruned graph (see Figure \ref{fig:mwst}).

\begin{figure}[htp]
    \centering
    \includegraphics[width=0.9\textwidth]{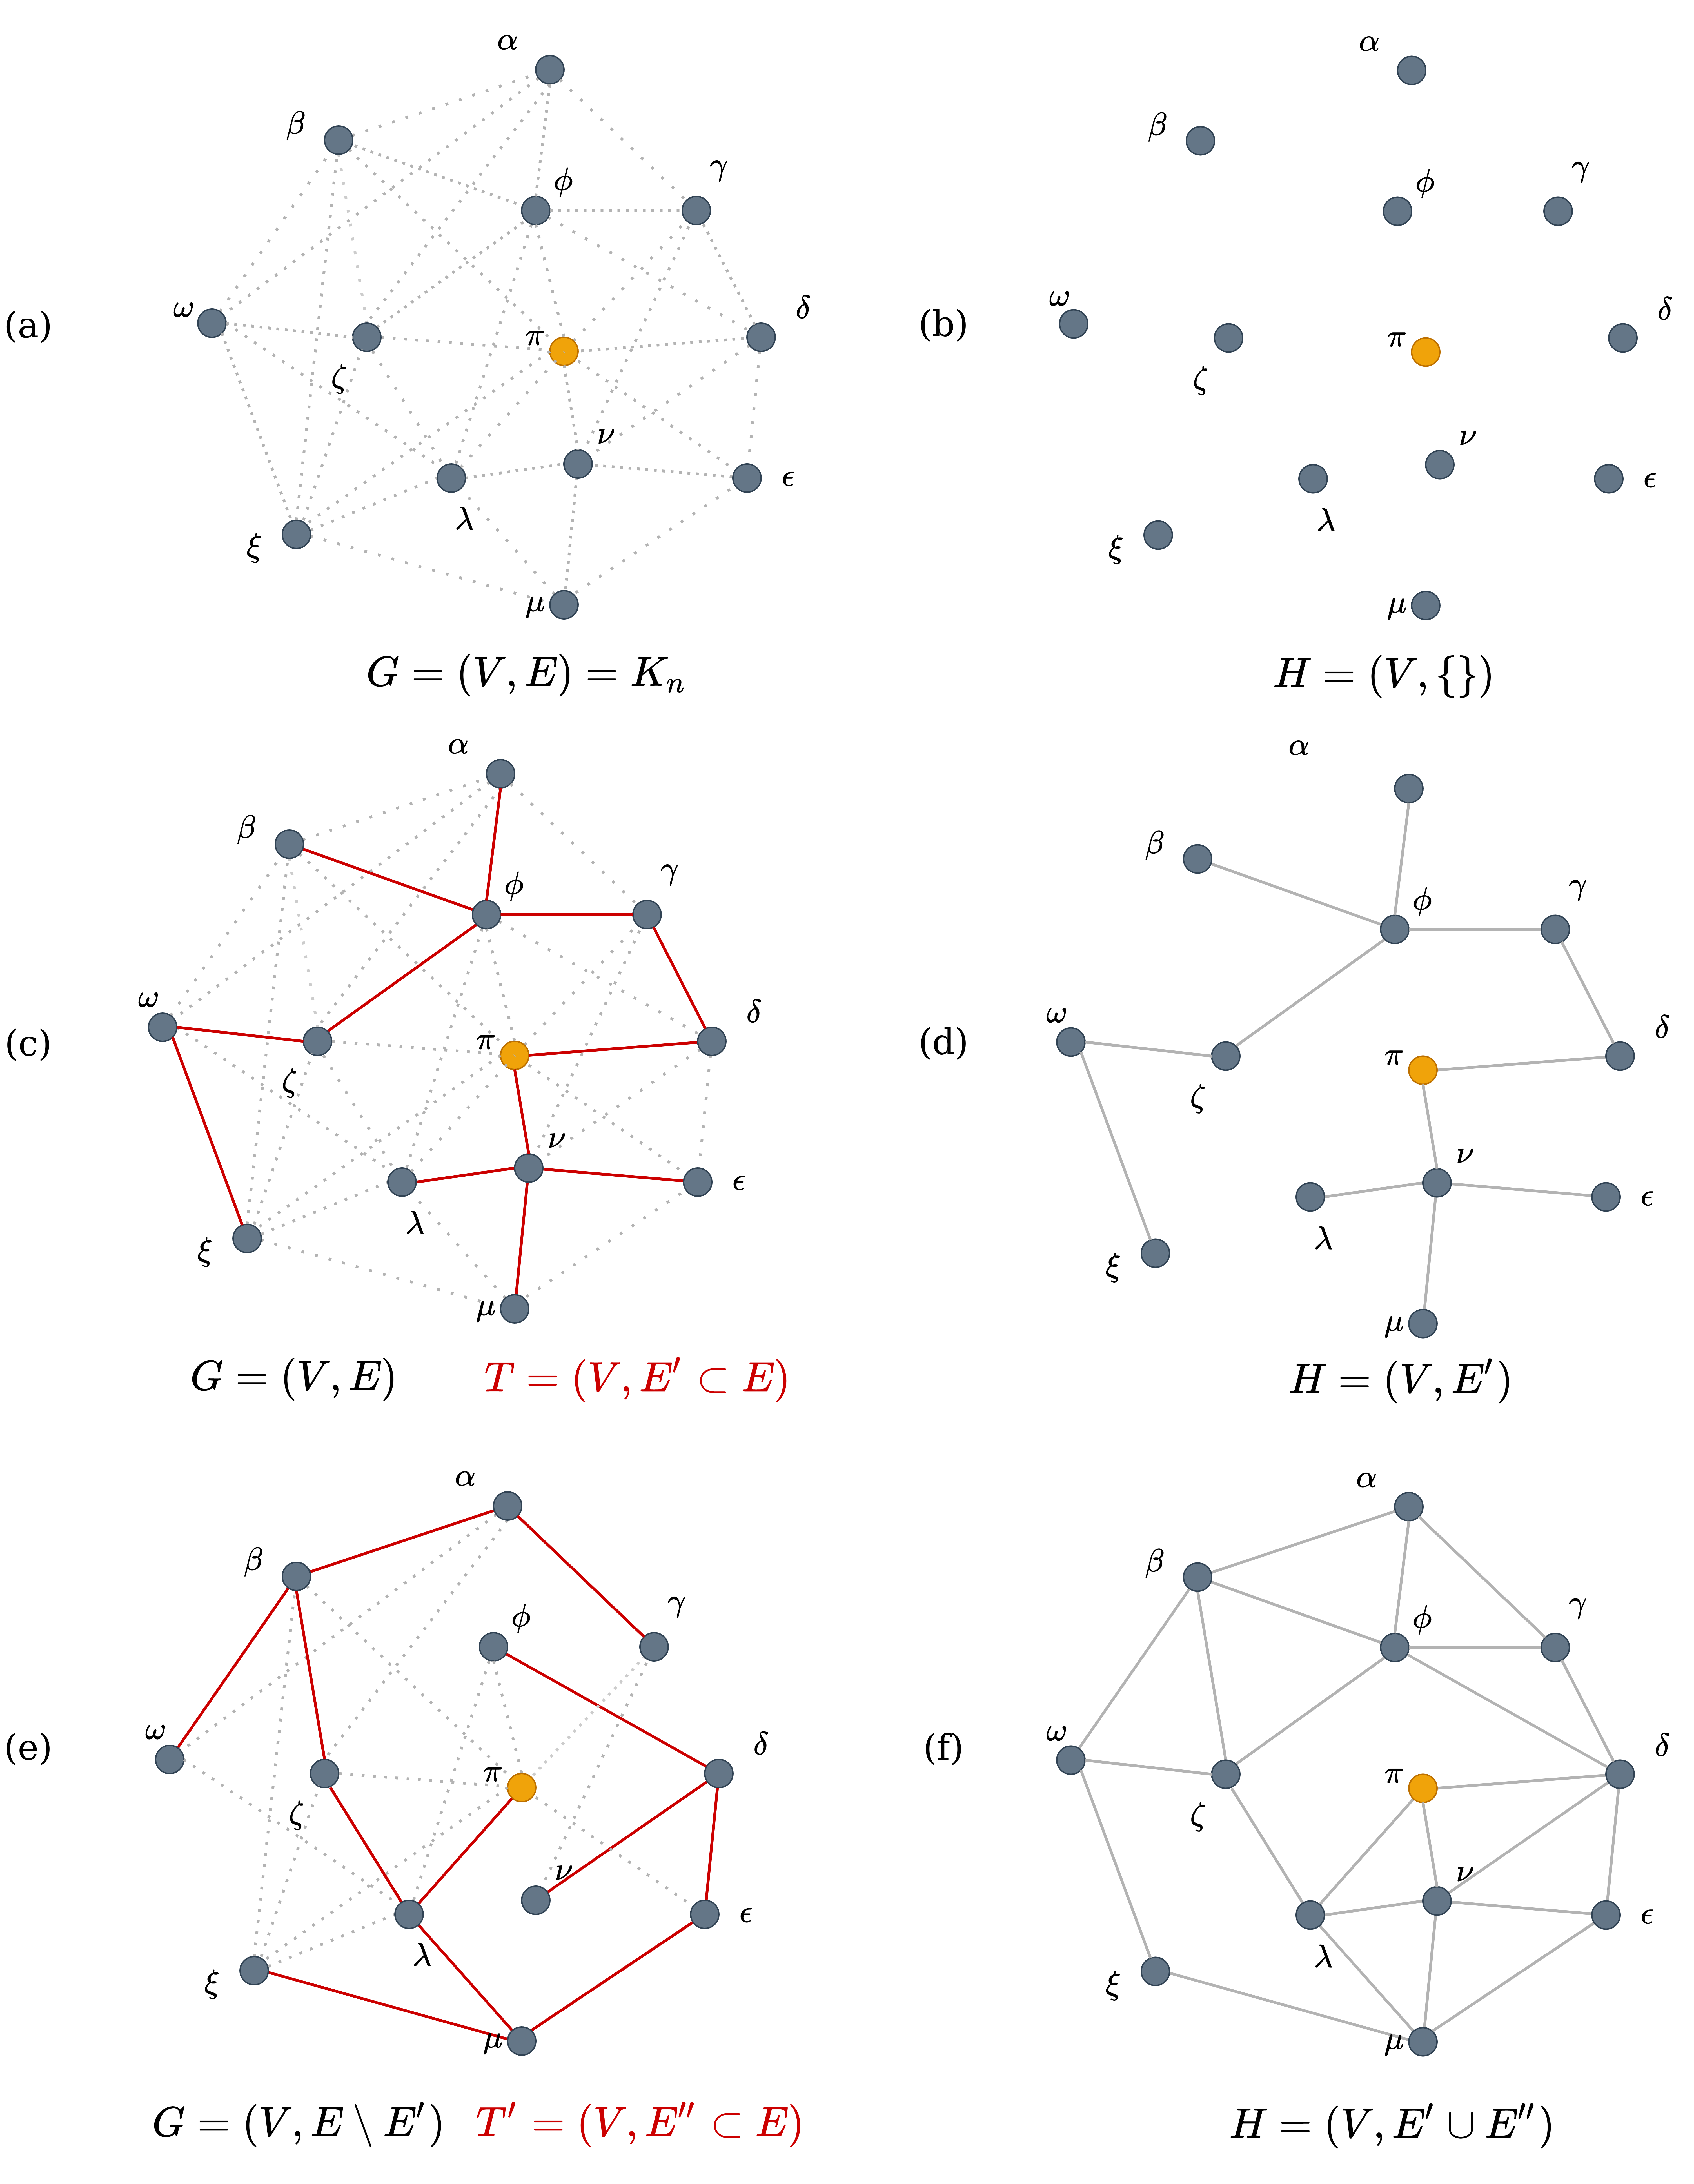}
    \caption{Extracting MWST edges for $k=2$ iterations. (a): The complete graph underlying the routing problem \footnote{In order to make the images easier to parse, many of the edges of the actual complete graph are not visualised}. (b): A new graph $H$ is initialised, that contains all of the vertices of $G$, but none of the edges. (c): The MWST $T$ of $G$ is computed. (d): The edges $E'$ are removed from $G$ and added to $H$. (e): A new MWST, $T'$, is computed from the modified graph $G$. (f): The edges $E''$ of the new tree $T$ are added to the graph $H$ and removed from $G$. We can also consider $H$ to be a sparsification of $G$.}
    \label{fig:mwst}
\end{figure}

\section{Doubletree Insertion}
\label{sec:dbtinsertion}

The doubletree approximation for a metric TSP constructs an approximate tour by computing a MWST in the underlying graph, duplicating the tree edges, visiting them in pre-order depth-first search and then removing the shortcuts from the pre-order list from left to right. In this work we compute a doubletour approximation in exactly this manner, but also construct another doubletour, creating shortcuts from right to left in the pre-order list. This gives two approximate tours, each guaranteed to have $\tilde{\ell} \leq 2$, with many overlapping edges. In practice this leads to slightly higher sacrifice in the pruning rate than a single tour does alone. Each time in this work it is stated that doubletour approximations are inserted into the pruned graph, it is actually these two doubletours, which increase slightly the chance for a pruned graph to admit better optimal solutions.

\end{subappendices}
